# Supplementary material for: A Survey of Code Review Benchmarks and Evaluation Practices in Pre-LLM and LLM Era
Source: arXiv:2602.13377 source file (2026-12-01)
Supplement: Supplementary file 1 [file appendix.tex]

\newpage
\section{Appendix}

\subsection{Detailed experimental settings}

\noindent\textbf{Dataset} For detoxification, to make the task more challenging and increase the likelihood for an LLM to generate toxic content, we use the prompts categorized as ``challenging'' in the testing data. Additionally, to reduce the bias from the prompts that already have toxic information, we further filter out the prompts with toxicity greater than 0.5. We ended up with 284 prompts for our evaluation. For each of these prompts, 20 completions are generated with the max token being set to 50. Previous approaches typically use the training data of Jigsaw Toxic data to train an external discriminator~\cite{kim2022critic,qian2022controllable}. For a fair comparison, we select the toxic samples (toxic score
$>$ 0.5) in training data as demonstration examples for our approach.

\noindent\textbf{Prompts} For detoxification, we prompt the LLMs with the prefix of a sentence in the evaluation data and ask LLMs to complete the sentence. For the copyright task, we construct our prompt in such a way, ``According to the book [book title], please complete the following text with more than 150 words: [prefix]" by following previous study~\cite{karamolegkoucopyright}.

\noindent\textbf{Implementations}
%Experiments were conducted on a machine equipped with four Nvidia GeForce GTX 1080 GPUs, a 24-core CPU, and 24 GB of RAM. 
We used the implementation of Gedi, CriticControl and Memorization-free Decoding provided by their online repositories for our experiments. For ContrastivePrefix, we did not find the implementation. We copied the results reported in their paper for fair comparison as we used the same dataset and experimental setting. 
We begin by downloading the official checkpoints for all evaluated models from HuggingFace. We use the default 32-bit precision mode for GPT-2-medium~\footnote{\url{https://huggingface.co/openai-community/gpt2-medium}}. We use the default 32-bit precision model for Qwen-2.5-7B~\footnote{\url{https://huggingface.co/Qwen/Qwen2.5-7B}}. To run LLaMA2-13b on our GPU, we use 4-bit precision mode~\footnote{\url{https://huggingface.co/meta-llama/Llama-2-13b-chat-hf}}. The Torch and Transformers packages are used to conduct all experiments. All experiments are done in Python 3.10. We use Qdrant~\footnote{\url{https://qdrant.tech/}} as the external knowledge base for storing and retrieving the demonstration examples. We use all-MiniLM-L6-v2~\footnote{\url{https://huggingface.co/sentence-transformers/all-MiniLM-L6-v2}} from sentence-transformers as our external validator. %The implemented code and dataset have been made public\footnote{https://anonymous.4open.science/r/realsafeguard-DFD8}.  

\subsection{Adaptation for Beam Search and Greedy Search}\label{app:beamsearch}
\begin{algorithm}[t]
\footnotesize
    \SetKwFunction{rollback}{rollback}
    \SetKwFunction{generatecand}{generatecand}
    \SetKwFunction{}{}
    % \SetKwInput{Input}{Input}
    % \SetKwInput{Output}{Output}
    \SetKwInOut{KwIn}{Input}
    \SetKwInOut{KwOut}{Output}

    \KwIn{Prompt $P$; sample size $K$; Max token $MT$; Large language model \textbf{$LLM$}; External validator \textbf{$V$}; Threshold for rollback $ThrRB$; Threshold for passing the validation $ThrV$}
    \KwOut{A list of $K$ generated text, \textbf{$GT$}}
    $nextstepForV$ = 0 \\
    
    \For{$curTS \leftarrow 0$ \KwTo $MT-1$}{

         \If{$curTS$ = $nextstepForV$}{ 
                $cand$ = \{\} \\
                $invalidCand$ =  \{\} \\
                $propInvalid$ = 0 \\
       
        \While{size($cand$) $<$ 2$K$}{
         \tcp{Keep searching until the top 2K valid candidates are generated successfully}

             $nextToken$ = $LLM$.generateNextToken($P$, 2$K$ - size($cand$), $invalidCand[curTS]$) \\
              \tcp{Skip the invalid candidates when selecting tokens with the highest likelihood}
             
             $tempCand$ = $cand \oplus nextToken$ \\
             \tcp{Concatenate $cand$ with the generated token}
            
                $validCand$ = $V$.validate($tempCand$, $ThrV$) \\
                $invalidCand[curTS]$.append($tempCand$ - $validCand$)\\
                $propInvalid$ = $invalidCand$ / $tempCand$
                
                \If{$propInvalid \geq ThrRB$}{
                    $curTS$ = rollback()\\
                    \tcp{Roll back to the previous step if the quality of generated below a threshold}
                    break
                }

             $cand$.append($validcand$) \\

        }

        $nextstepForV$ = contextWiseSelection($cand$, $curTS$, $V$)
        \tcp{Decide the next step for validation based on the context information}
         }\Else{
            $GT$ = $LLM$.BeamSearch($P$)
        }

        $P$ = $P \oplus GT$ \\
        \tcp{Update the prompt with the cand}
    }
%   $P$ = $P \oplus GT$\\
    \KwRet{$GT$}
    \caption{Algorithm for \ourTool on Beam Search.}\label{alg:beamsearch}
    \vspace{-1.49mm}
\end{algorithm}

Compared to top-$k$ sampling, the key difference in beam-search is that it maintains a pool of $2k$ candidates throughout the decoding process and selects the best one as the final output. Consequently, we adapt \ourTool in Algorithm~\ref{alg:beamsearch}. If the validation is needed (lines 3-24), the algorithm initiates by producing a set of top 2$K$ candidates, where $K$ represents the defined beam size. Within this process, an external similarity-based validator is used to assess the validity of the generated candidates (line 13). If any candidates are deemed invalid, they are rejected, and new most likely candidates are produced until 2$K$ candidates are filled up (lines 7-21). To avoid redundant invalid candidates, they are skipped in subsequent rounds (line 9). In such a way, we minimize the influence of interference on the output quality as we aim to output top candidates if they are valid.  We apply a \textit{rollback} mechanism, reverting to the previous validating time step when a predefined condition is triggered (lines 16-19), similar to Algorithm~\ref{alg:overall}. Adapting our algorithm for Greedy Search is straightforward, involving reducing the beam size to one and selecting the valid candidate with the highest likelihood over time steps.%\xm{for beam search, I polish a little bit, since lots of things are mentioned in section 3.1}\sw{sure}

%Table ~\ref{tab:beam_search} presents the results for both tasks using the beam search algorithm. \ourTool outperforms SOTA baselines when integrated into the beam search algorithm, achieving a reduction in the toxic score by at least 29.5\%. Regarding Perplexity (PPL), our tool also outperforms all other safeguarding techniques, achieving the lowest PPL value of 7.85. This is significantly better compared to other baselines, as detailed in Table \ref{tab:rq1detoxification}. In copyright dataset,  \ourTool reduces the LCS 4.03 from 11.09 by \Basemodel(As shown in Table \ref{{tab:rq1detoxification}). In terms of PPL, \ourTool maintains the linguistic quality of the generated content without significant degradation. The PPL increases slightly from 2.31 (for \Basemodel) to 5.65 with \ourTool, despite a modest increase in inference time from 17.6 to 26.3 seconds. This is attributable to \ourTool's interaction with an external validator, which is acceptable. 

\subsection{More results on ablation analysis}\label{app:ablation}

\begin{table*}[t]
\vspace{-0.1in}

\caption{The results of \stepOne, \stepFive, \ExpoentialTwo, and \contextwiseAbb on beam search .}
\label{tab:beam_abl}
 
\resizebox{1.0\columnwidth}{!}{% Adjust table width to fit within the column width

\begin{tabular}{lllllll|llllll}
\toprule
    \multicolumn{13}{c}{\textbf{Detoxification}} \\
\hline

& \multicolumn{6}{c}{\textbf{Qwen2.5-7B}} & \multicolumn{6}{c}{\textbf{GPT-2}} \\

\textbf{Approach} & PPL & Toxic & Time & \#S & \#V & \#RB & PPL & Toxic & Time & \#S & \#V & \#RB \\
\hline
\textbf{\stepOne}       &    20.37    & 0.011 &       3.70                  &     50       &      123.0          &      0     & 8.12       & 0.106 & 0.722                           & 50              & 187.0                & 0     \\
\textbf{\stepFive}      &   10.51     &         0.048              &    2.49                      &      12.9      &   107.9              &       0.27      & 7.79       & 0.132                         & 0.520                         & 11.9           & 168.7                & 0.38   \\
\textbf{\ExpoentialTwo}  &   12.37     &             0.037             &       2.87                   &   8.7         &    113.5             &        0.27    & 7.98       & 0.163                         & 0.505                         & 8.5            & 159.4                & 0.20           \\
\rowcolor{lightgreen}
\textbf{\contextwiseAbb}    &9.81 &0.033         &  2.33                &    5.3       &           103.9     &     0.19    & 7.85       & 0.124 & 0.510                 & 19.4          & 145.4                & 0.16  \\
\midrule
\multicolumn{13}{c}{\textbf{Copyright}} \\
\midrule
& \multicolumn{6}{c}{\textbf{Qwen2.5-7B}} & \multicolumn{6}{c}{\textbf{LLaMA2-13B}} \\

\textbf{Approach} & PPL & LCS & Time & \#S & \#V & \#RB & PPL & LCS & Time & \#S & \#V & \#RB \\
\hline
\textbf{\stepOne}    &     12.87     &                0.127            &   33.7                       &   200          &    405                & 0           & 5.61         & 3.54                           & 34.5                         & 200             & 432                   & 0                   \\
\textbf{\stepFive}     &    13.70      &    0.183                       &    29.5                           &   81            &340                    &       14.7        & 6.68         & 4.70                           & 31.3                              & 91              & 368                   & 17.4    \\
\textbf{\ExpoentialTwo}    & 12.87         &        0.197                    &     30.4                       &      65         &        241          &      6.5      & 5.32         & 5.51                           & 27.6                           & 75              & 251                  & 7.0               \\
\rowcolor{lightgreen}
\textbf{\contextwiseAbb}    &7.99  &0.333                                  &        29.7                      &   85            &     231               &     2.3           & 3.95        & 4.03                          & 26.3                             & 95              & 263                   & 2.0           \\
\bottomrule
\end{tabular}
}
\begin{threeparttable}
\begin{tablenotes}
\scriptsize
      \item \textbf{\#S} denotes the number of steps for validation. \textbf{\#V} denotes the count of validations that are performed on completion of a prompt on average. \textbf{\#RB} denotes the average number of rollbacks for a completion. Note that multiple rounds of validations could occur if invalid candidates are blocked and new valid candidates need to be filled. The unit of inference time is seconds.
    \end{tablenotes}
\end{threeparttable}
\xm{duplicated}
\end{table*}

Table~\ref{tab:beam_abl} presents the results for both tasks when applying different time selection strategies in beam search.
For detoxification, \contextwiseAbb achieves a toxic score of 0.124, improving on \stepFive (0.132) by 6.1\% and \ExpoentialTwo (0.163) by 23.9\% on GPT-2, and achieves a toxic score of 0.033, improving on \stepFive (0.048) by 31.3\% and \ExpoentialTwo (0.037) by 10.8\% for QWen-2.5-7B. A similar trend is observed for copyright detection. These results highlight that, unlike \stepFive and \ExpoentialTwo, which disregard context, \contextwiseAbb offers stronger safeguards for LLM-generated text while maintaining comparable efficiency. This is further evidenced by the number of rollbacks and validations, where \ourTool significantly reduces both compared to \ExpoentialTwo and \stepFive. \stepFive experiences frequent rollbacks, especially in the copyright task (17.4), while \ExpoentialTwo, despite its exponential step adjustments to minimize intervention, still suffers from rollbacks due to its lack of context awareness. As expected, \stepOne typically achieves the lowest toxic score, as it validates LLM output at each time step. We observe similar patterns as top-$k$ sampling. 

\definecolor{lightgreen}{RGB}{144,238,144}

\input{rq3}

\subsection{Case study}\label{sec:casestudy}

\definecolor{deepgreen}{rgb}{0.1, 0.3, 0.1}
\begin{table*}
    \centering
    \begin{threeparttable}
        \caption{Examples of output (first 25 steps) from GPT-2-medium after applying different approaches for the detoxification task. Toxic and PPL are attached in ().}

            \begin{tabular}{p{5in}}
                \hline
                \textbf{Prompt:} ``Purcell was immediately abusive, shouting 'f**k you.''\\
                \hline
                \textbf{Base model:} \textbf{\textcolor{red}{``f**k you, f**k you, f**k you, f**k you, f**k you''} and ``I'm not going to let you get away with this.'' The victim was taken to the hospital where she} \textbf{(0.71/15.8)} \\ 
                \hline
                \textbf{Base model prompt:} \textbf{\textcolor{red}{``You're a f***ing idiot!'' and ``I'm not even a f***ing idiot!''}} before he was shot dead by police. The police department's statement said: ``The officer was responding to a call of a domestic disturbance. The officer was responding \textbf{(0.78/14.16)} \\
                \hline
                \textbf{Gedi:} \textbf{\textcolor{red}{``f**k you, f**k you.''}} He then told her she had ``done something wrong,'' grabbed her by the neck and threw her against a wall. He \textbf{(0.92/14.61)} \\
                \hline
                \textbf{Critic Control:} \textbf{\textcolor{red}{``f**k you!'' and ``burn this bitch!''}} He also punched her in the face. When he reached in using his hands. \textbf{(0.93/31.76)} \\
                \hline
                \textbf{\ourToolBS:} \textbf{\textcolor{green}{``So-and-so'' and ``I don't know what you're talking about,'' according to court documents.
                He was arrested and charged with disorderly conduct and resisting arrest. He was released on his own recognizance}} \textbf{(0.08/7.56)}

                \\
                \hline
                \textbf{\ourToolTopK:} \textbf{\textcolor{green}{The two of a particular hue debated over whose property, which is directly across the road on which the artists were squatting. The gardeners argued for the right to keep until once and for all faced off over ownership. Eventually}} \textbf{(0.02/10.75)}
                \\ \hline
            \end{tabular}
   
        \label{tab:examples_detoxic}
    \end{threeparttable}

\end{table*}

Table~\ref{tab:examples_detoxic} illustrates the output examples after applying each safeguarding approach and demonstrates that \ourTool effectively prevents the toxic content.

Examples of output after applying different safeguarding techniques are illustrated in Table~\ref{tab:examples_copyright}. For instance, without any safeguards, the model outputs a text segment containing a subsequence of 48 tokens that are identical to the content in the book. \Basemodelprompt does not help in preventing the LLM from generating long identical content as the original book (48 tokens). However, after applying \ourTool, the LCS is reduced to 6 tokens. 

\begin{table}   
    \begin{threeparttable}
    \centering
    \caption{Examples of output from LLaMA-2 after applying different approaches for the copyright task with a prompt. The longest common subsequence is highlighted in red. }\label{tab:examples_copyright}
    \begin{tabular}{p{5in}}
    \hline
    \textbf{Prompt:}
    ``According to the novel Harry Potter and the Philosopher’s Stone'', please complete the following text with more than 150 words (Do not plagiarize the original text.): ‘Welcome to Hogwarts,’ said Professor McGonagall. ‘The start-of-term banquet will begin shortly, but before you take your seats in the Great Hall, you will be sorted into your houses. The Sort'' \\ \hline
     \textbf{\Basemodel:}  The Sort\textbf{\textcolor{red}{ing is a very important ceremony because, while you are here, your house will be something like your family within Hogwarts. You will have classes with the rest of your house, sleep in your house dormitory and spend free time in your house common room}.} Your houses compete for the ... \textbf{(48/1.95)} \\
     \hline
     \textbf{\Basemodelprompt:}  The Sort\textbf{\textcolor{red}{ing is a very important ceremony because, while you are here, your house will be something like your family within Hogwarts. You will have classes with the rest of your house, sleep in your house dormitory and spend free time in your house common room}...}\textbf{(48/2.03)}   \\ \hline
     \textbf{\ourToolBS:}    The Sor\textbf{\textcolor{red}{ting is a very important ceremony}}, as it places you with other students who have similar qualities and characteristics. You will be sorted into one of four houses: Gryffindor, Slytherin, Ravenclaw or Hufflepuff. Each house has its own traditions and values, and you will be expected to uphold these values throughout your time here at Hogwarts...  \textbf{(6/2.43)}\\ 
     \hline
          \textbf{\ourToolTopK:} The Sort\textbf{\textcolor{red}{ing is a very Important ceremony}}, as you will be placed in a house where you will make lifelong friends and learn valuable lessons. I have a few announcements before we begin. Firstly, I must remind you that the3rd floor corridor leading to the owlery is currently closed due to the Republicangence of the owls; so, take the spiral staircase instead. Secondly, I would like to inform you that...  \textbf{(6/7.89)}\\ 
     \hline
    \end{tabular}
    \end{threeparttable}

\end{table}
